# Supplementary material for: Internal dynamics and dielectric screening of confined multiexciton states
Source: arXiv:2507.11087 ancillary file (2025-07-15)
Supplement: Supplementary file 1 [file SuplementariMaterial.pdf]

# Internal dynamics and dielectric screening of confined multiexciton states - Supplemental Material


Josep Planelles, Juan I. Climente

*Dept. de Química Física i Analítica,*

*Universitat Jaume I, 12080, Castelló, Spain*

José L. Movilla

*Dept. d'Educació i Didàctiques Específiques,*

*Universitat Jaume I, 12080, Castelló, Spain*[*]



(Dated: July 15, 2025)



[*]Electronic address: movilla@uji.es

**Characteristic Frequency of the harmonic oscillator and the hydrogen atom**

The characteristic frequency $\omega$ and the energy of the fundamental transition $0 \rightarrow 1$ of the harmonic oscillator, $E_1 - E_0 = \hbar\omega$, are the same, except for a factor, $\hbar$, which converts frequency to energy units.

In the case of a hydrogen-like system, such as an exciton (electron-hole), the virial theorem for the Coulomb potential $V(r) \propto -\frac{1}{r}$ states that the average kinetic energy $\langle T\rangle$ and the average potential energy $\langle V\rangle$ are related: $2\langle T\rangle + \langle V\rangle = 0$, with $\langle(T+V)\rangle = E$. In the case of the ground state we then deduce that: $\langle T\rangle = -E_0 = E_b$, where $E_b = -E_0$ is the binding energy. Assuming that the kinetic energy comes mainly from the relative motion of the particles, we can find the relative velocity:

$$T = \frac{1}{2}\mu v^2 = E_b \quad \Rightarrow \quad v = \sqrt{\frac{2E_b}{\mu}}.$$

And if we identify the characteristic frequency $\omega$ of the exciton with $v/r$, determine the binding energy $E_b$ and the radius $r$ using the Bohr model,

$$E_b = \frac{\mu e^4}{2(4\pi\epsilon_0\epsilon)^2\hbar^2} \quad ; \quad r = \frac{4\pi\epsilon_0\epsilon\hbar^2}{\mu e^2} \Rightarrow \quad r = \frac{\hbar}{\sqrt{2\mu E_b}}.$$

and substituting $v$ and $r$ from the previous expressions we obtain the characteristic frequency in terms of the binding energy:

$$\omega = \frac{v}{r} = \frac{\sqrt{\frac{2E_b}{\mu}}}{\frac{\hbar}{\sqrt{2\mu E_b}}} = \frac{2E_b}{\hbar}.$$

On the other hand, following the oscillator analogy, we now calculate the frequency of the fundamental transition:

$$\omega = \frac{E_1 - E_0}{\hbar} = \frac{3}{4}\frac{E_b}{\hbar}.$$

Although, as we can see, there is no *exact* correspondence between one frequency and the other as there was in the oscillator case, we can define a *characteristic frequency* $\omega$ as the ratio between the *characteristic energy* $E_b$ and $\hbar$: $\omega = E_b/\hbar$. Alternatively, and more generally, we can find the quantum mechanical expectation value of $\frac{v}{r}$ in the state we are interested in studying.

**Effective Field Fluctuation Frequency**

We can associate to each system or subsystem of two interacting particles an **effective field fluctuation frequency** $\omega_{\text{eff}} \sim \frac{v}{r}$, where $v$ is the relative velocity and $r$ the distance between the particles. We define the relative velocity as $v = p_r/\mu$, and hence try to find the quantum mechanical operator associated with $\omega_{\text{eff}}$.

The quantum mechanical operator associated with $p_r$ is:[1, 2]

$$\hat{p}_r = -i\hbar \frac{1}{r}\frac{\partial}{\partial r} r$$

The non-commutativity of $\hat{p}_r$ and $r$ leads us to define the Hermitian operator associated with $\frac{\hat{p}_r}{\mu\, r}$ as:

$$\hat{\omega}_{\text{eff}} = \widehat{\frac{p_r}{\mu r}} = \frac{1}{2\mu}\left(\frac{1}{r}\hat{p}_r + \hat{p}_r\frac{1}{r}\right) = -\frac{i\hbar}{\mu}\left(\frac{1}{r}\frac{\partial}{\partial r} + \frac{1}{2r^2}\right)$$

Therefore, we must compute $\langle\Phi|\hat{\omega}_{\text{eff}}(r)|\Phi\rangle$ in the excitonic case, while in the trionic and biexcitonic cases, we should compute $\langle\Phi|\hat{\omega}_{\text{eff}}(r_{e1-h1})|\Phi\rangle$.

As a guideline, we can approximate the integrals by considering the independent-particle part as constant under the derivative involved in $\omega_{\text{eff}}$, so that we only differentiate the Jastrow factor with respect to $r_{e1-h1}$. In particular, for the exciton, assuming the vacuum dielectric constant, this amounts to computing $\omega_{\text{eff}}$ using the ground state $R_{1,0} = 2e^{-r}$ of the hydrogen atom:

$$\langle\hat{\omega}_{\text{eff}}\rangle = -\frac{i\hbar}{\mu}\int_0^\infty 2e^{-r}\left(\frac{1}{r}\frac{\partial\, 2e^{-r}}{\partial r} + 2e^{-r}\frac{1}{2r^2}\right) r^2 dr = 0$$

As we see, there is no net radial flux. The electron has no preferred motion inward or outward. The wavefunction $R_{1,0} = 2e^{-r}$ is radial and spherically symmetric. Positive and negative fluctuations of the momentum cancel, yielding a result of zero.

We can instead compute the square of the effective frequency operator and then take the square root. We thus consider the operator:

$$\omega^2_{\text{eff}} = -\frac{\hbar^2}{\mu^2}\left(\frac{1}{r}\frac{\partial}{\partial r} + \frac{1}{2r^2}\right)^2$$

and the wavefunction $R_{1,0} = 2e^{-r}$. In doing this, we encounter another hurdle: the integral involved in computing $\langle\omega^2_{\text{eff}}\rangle$ is divergent. The divergence arises from the $1/r^2$ singularity in $\hat{\omega}^2_{\text{eff}}$ at $r = 0$, typical for $s$-states. This indicates that the dispersion (or variance) of this operator

in the ground state does not exist (it is infinite). This is why in the main text we seek for an alternative and extract frequencies from the **variance:**

$$\omega_A = \frac{\sqrt{\langle [\hat{H}, \hat{A}]^2 \rangle}}{\hbar \sqrt{\langle \hat{A}^2 \rangle}},$$

**Toy-example: Characteristic Frequency from the Variance in the Ground State of the Hydrogen Atom**

Let us consider the operator $\hat{A} = r$ (radial distance) and define $\hat{\Omega}_r = \frac{i}{\hbar}[\hat{H}, r]$.
The Hamiltonian of the hydrogen atom in atomic units ($\hbar = m = e = 1$) is:

$$\hat{H} = -\frac{1}{2}\nabla^2 - \frac{1}{r},$$

From $[\hat{H}, r] = -\frac{i}{m}\hat{p}_r$, with $\hat{p}_r = -i\left(\frac{\partial}{\partial r} + \frac{1}{r}\right)$ the radial momentum operator, and taking $m = 1$ a.u., we obtain:

$$\hat{\Omega}_r = \frac{i}{\hbar}[\hat{H}, r] = \hat{p}_r.$$

The expectation value and variance of $\hat{\Omega}_r = \hat{p}_r$ in the normalized ground-state wavefunction, $R_{10}(r) = 2e^{-r}$, are:

- Expectation value: $\langle \hat{p}_r \rangle = 0$.
- Variance: $\Delta p_r = \sqrt{\langle \hat{p}_r^2 \rangle - \langle \hat{p}_r \rangle^2} = \sqrt{\langle \hat{p}_r^2 \rangle}$.

Using $\hat{p}_r^2 = -\left(\frac{d^2}{dr^2} + \frac{2}{r}\frac{d}{dr}\right)$, the expectation value becomes:

$$\langle \hat{p}_r^2 \rangle = \int_0^\infty R_{10}^*(r)\hat{p}_r^2 R_{10}(r) r^2 dr,$$

For the hydrogen ground state, $l = 0$, we have $\langle \hat{p}_r^2 \rangle = \langle \hat{p}^2 \rangle$, and in atomic units, $\langle \hat{p}^2 \rangle = \langle \psi_{1s}| - \nabla^2 |\psi_{1s}\rangle = 1$. Therefore, $\langle \hat{p}_r^2 \rangle = 1$. Similarly, we compute $\langle r^2 \rangle = 3$.
The "frequency" associated with $\hat{\Omega}_r = \hat{p}_r$ is thus: $\omega = \frac{\sqrt{\langle \hat{p}_r^2 \rangle}}{\sqrt{\langle r^2 \rangle}} = \frac{1}{\sqrt{3}} = 0.577 \quad \text{(a.u.)}$.
In atomic units, the ground-state energy is $E_0 = -\frac{1}{2}$, and the characteristic energy frequency is $\frac{|E_0|}{\hbar} = \frac{1/2}{1} = 0.5$ a.u., while the magnitude of the variance of the radial momentum we computed is about 0.6, which is consistent as an order of magnitude.
If we use an approximate wavefunction $\Psi = 2a^{2/3}\, e^{-ar}$, which could represent a Jastrow-type

correlation factor for a confined exciton, we obtain $\langle \hat{p}_r^2 \rangle = a^2$, $\langle r^2 \rangle = \frac{3}{a^2}$, which gives a frequency (in a.u.) $\omega = \frac{a^2}{\sqrt{3}}$.

### Characteristic frequency of confined exciton, trion, and biexciton

We want to calculate the characteristic frequency of the electron-hole relative motion inside a three-dimensionally confined *effective exciton.* This frequency is defined as:

$$\omega_A = \frac{\sqrt{\langle [\hat{H}, \hat{A}]^2 \rangle}}{\hbar \sqrt{\langle \hat{A}^2 \rangle}},$$

where $\hat{A} = \mathbf{r}_1 - \mathbf{R}_a$ is the relative position operator between an electron and a hole.
The elements for calculating $\omega_A$ are the denominator $\langle r_{1a}^2 \rangle$, whose expectation value is straightforward,

$$\langle \hat{A}^2 \rangle = \langle r_{1a}^2 \rangle = \int d\mathbf{r}_1 \cdots d\mathbf{R}_b \, |\Psi|^2 \, r_{1a}^2,$$

and the numerator $\langle [\hat{H}, \hat{A}]^2 \rangle$, which, as we saw in the main text, can be interpreted as the expectation of the local observable:

$$O(\Psi(\mathbf{X})) = \left| \frac{1}{m_e} \nabla_1 \ln \Psi(\mathbf{X}) - \frac{1}{m_h} \nabla_a \ln \Psi(\mathbf{X}) \right|^2,$$

over the probability distribution $\Psi^2(\mathbf{X})$.

### Local Observable for an Exciton Confined in a Box

Consider an exciton formed by an electron at position $\mathbf{r}_1 = (x_1, y_1, z_1)$ and a hole at position $\mathbf{R}_a = (X_a, Y_a, Z_a)$, with wavefunction:

$$\Psi(\mathbf{r}_1, \mathbf{R}_a) = \psi_{\text{box}}(\mathbf{r}_1) \, \psi_{\text{box}}(\mathbf{R}_a) \, e^{-z r_{1a}},$$

where $r_{1a} = |\mathbf{r}_1 - \mathbf{R}_a|$, and $\psi_{\text{box}}(\mathbf{r}) = \cos(k_x x) \cos(k_y y) \cos(k_z z)$.

To implement it in a standard Metropolis algorithm, we decompose the observable as:

$$O(\Psi(\mathbf{X})) = \sum_{\mu = x,y,z} \left( \frac{1}{m_e} \frac{\partial \ln \Psi}{\partial r_{1\mu}} - \frac{1}{m_h} \frac{\partial \ln \Psi}{\partial R_{a\mu}} \right)^2.$$

**Logarithmic Derivatives of the Wavefunction**

We calculate each derivative as:

$$\frac{\partial \ln \Psi}{\partial r_{1\mu}} = \frac{\partial \ln \psi_{\text{box}}}{\partial r_{1\mu}} - z\frac{\partial r_{1a}}{\partial r_{1\mu}}, \quad \frac{\partial \ln \Psi}{\partial R_{a\mu}} = \frac{\partial \ln \psi_{\text{box}}}{\partial R_{a\mu}} - z\frac{\partial r_{1a}}{\partial R_{a\mu}}.$$

where

$$\frac{\partial r_{1a}}{\partial r_{1\mu}} = \frac{r_{1\mu} - R_{a\mu}}{r_{1a}}, \quad \frac{\partial r_{1a}}{\partial R_{a\mu}} = \frac{R_{a\mu} - r_{1\mu}}{r_{1a}} = -\frac{\partial r_{1a}}{\partial r_{1\mu}}.$$

**Logarithmic Gradient of the Confinement Factor**

$$\frac{\partial \ln \psi_{\text{box}}}{\partial r_{1\mu}} = -k_\mu \tan(k_\mu r_{1\mu}), \quad \frac{\partial \ln \psi_{\text{box}}}{\partial R_{a\mu}} = -k_\mu \tan(k_\mu R_{a\mu}).$$

**Final Result**

Substituting all into the observable expression:

$$O(\Psi(\mathbf{X})) = \sum_{\mu=x,y,z} \left[ -\frac{k_\mu}{m_e} \tan(k_\mu r_{1\mu}) + \frac{k_\mu}{m_h} \tan(k_\mu R_{a\mu}) - z\left(\frac{1}{m_e} + \frac{1}{m_h}\right) \frac{r_{1\mu} - R_{a\mu}}{r_{1a}} \right]^2.$$

This expression can be evaluated in a VQMC code, using samples generated according to the density $|\Psi|^2$.

**Local Observable for a Confined Trion $X^*$ in a Box**

The trion $X^*$ wavefunction is:

$$\Psi_{X^*} = \phi(\mathbf{r}_{e1}) \cdot \phi(\mathbf{r}_{e2}) \cdot \phi(\mathbf{r}_h) \cdot J(r_1, r_2, r_{12}),$$

with $\phi(\mathbf{r}) = \cos(k_x x_i) \cos(k_y y_i) \cos(k_z z_i)$ and $J(r_1, r_2, r_{12})$ the Jastrow factor:

$$J(r_1, r_2, r_{12}) = e^{-Zs/2} \cosh\left(\frac{ZQt}{2}\right) e^{\frac{Zbr_{12}}{1+Zar_{12}}},$$

where

$$r_1 = |\mathbf{r}_{e1} - \mathbf{r}_h|, \quad r_2 = |\mathbf{r}_{e2} - \mathbf{r}_h|, \quad r_{12} = |\mathbf{r}_{e1} - \mathbf{r}_{e2}|, \quad s = r_1 + r_2, \quad t = r_1 - r_2.$$

The local observable is:

$$O(\Psi(\mathbf{X})) = \left| \frac{1}{m_e} \nabla_1 \ln \Psi - \frac{1}{m_h} \nabla_h \ln \Psi \right|^2 .$$

**Logarithmic Derivatives**

We use:

$$\nabla_i \ln \Psi = \nabla_i \ln \phi_i + \nabla_i \ln J,$$

and for the $\phi$ part,

$$\partial_{r_{i,\mu}} \ln \phi(\mathbf{r}_i) = -k_\mu \tan(k_\mu r_{i,\mu}).$$

**Derivative of** $\ln J$

We have:

$$\ln J = -\frac{Zs}{2} + \ln \cosh\left(\frac{ZQt}{2}\right) + \frac{Zbr_{12}}{1 + Zar_{12}}$$

*Gradient with respect to* $\mathbf{r}_{e1}$*:*

$$\nabla_1 r_1 = \frac{\mathbf{r}_{e1} - \mathbf{r}_h}{r_1}, \quad \nabla_1 r_2 = 0, \quad \nabla_1 r_{12} = \frac{\mathbf{r}_{e1} - \mathbf{r}_{e2}}{r_{12}}$$

$$\nabla_1 s = \frac{\mathbf{r}_{e1} - \mathbf{r}_h}{r_1}, \quad \nabla_1 t = \frac{\mathbf{r}_{e1} - \mathbf{r}_h}{r_1}$$

$$\nabla_1 \left(-\frac{Zs}{2}\right) = -\frac{Z}{2} \frac{\mathbf{r}_{e1} - \mathbf{r}_h}{r_1}$$

$$\nabla_1 \ln \cosh\left(\frac{ZQt}{2}\right) = \frac{ZQ}{2} \tanh\left(\frac{ZQt}{2}\right) \frac{\mathbf{r}_{e1} - \mathbf{r}_h}{r_1}$$

$$\nabla_1 \left(\frac{Zbr_{12}}{1 + Zar_{12}}\right) = \left(\frac{Zb}{(1 + Zar_{12})^2}\right) \frac{\mathbf{r}_{e1} - \mathbf{r}_{e2}}{r_{12}}$$

$$\nabla_h t = \nabla_h r_1 - \nabla_h r_2 = \frac{\mathbf{r}_h - \mathbf{r}_{e1}}{r_1} - \frac{\mathbf{r}_h - \mathbf{r}_{e2}}{r_2} = -\left(\frac{\mathbf{r}_{e1} - \mathbf{r}_h}{r_1} - \frac{\mathbf{r}_{e2} - \mathbf{r}_h}{r_2}\right)$$

Thus, the derivative of the cosh term is:

$$\begin{aligned}\nabla_h \ln\cosh\left(\frac{ZQt}{2}\right) &= \frac{ZQ}{2}\tanh\left(\frac{ZQt}{2}\right)\nabla_h t \\ &= -\frac{ZQ}{2}\tanh\left(\frac{ZQt}{2}\right)\left(\frac{\mathbf{r}_{e1} - \mathbf{r}_h}{r_1} - \frac{\mathbf{r}_{e2} - \mathbf{r}_h}{r_2}\right)\end{aligned}$$

With all of this, the explicit formula for the observable to implement is:

$$\begin{aligned}O(\Psi(\mathbf{X})) = \sum_{\mu=x,y,z}\Bigg\{&\frac{1}{m_e}\left(-k_\mu \tan(k_\mu r_{e1,\mu})\right) - \frac{1}{m_h}\left(-k_\mu \tan(k_\mu r_{h,\mu})\right) \\ &+ \frac{1}{m_e}\left(-\frac{Z}{2} + \frac{ZQ}{2}\tanh\left(\frac{ZQt}{2}\right)\right)\frac{r_{e1,\mu} - r_{h,\mu}}{r_1} \\ &+ \frac{1}{m_e}\left(\frac{Zb}{(1+Zar_{12})^2}\right)\frac{r_{e1,\mu} - r_{e2,\mu}}{r_{12}} \\ &- \frac{1}{m_h}\left(\frac{Z}{2} - \frac{ZQ}{2}\tanh\left(\frac{ZQt}{2}\right)\right)\frac{r_{e1,\mu} - r_{h,\mu}}{r_1} \\ &- \frac{1}{m_h}\left(\frac{Z}{2} + \frac{ZQ}{2}\tanh\left(\frac{ZQt}{2}\right)\right)\frac{r_{e2,\mu} - r_{h,\mu}}{r_2}\Bigg\}^2\end{aligned}$$

### The Local Observable for a Biexciton $BX$ Confined in a Box

The wave function of the biexciton has the form:

$$\Psi = \prod_{i=a,b,1,2}\cos(k_x x_i)\cos(k_y y_i)\cos(k_z z_i) \times F(r_{1a}, r_{1b}, r_{2a}, r_{2b})$$

$$F = e^{-Z\frac{s_1+s_2}{2}}\cosh\left[ZQ\frac{t_1 - t_2}{2}\right] e^{Z\frac{\beta r_{12}}{1+Z\alpha r_{12}}} e^{Z\frac{\beta r_{ab}}{1+Z\alpha r_{ab}}},$$

with the definitions:

$$s_1 = r_{1a} + r_{1b}, \quad s_2 = r_{2a} + r_{2b}, \quad t_1 = r_{1a} - r_{1b}, \quad t_2 = r_{2a} - r_{2b}.$$

For the implementation with a standard Metropolis algorithm, we wrote the observable as:

$$O(\Psi(\mathbf{X})) = \sum_{\mu=x,y,z}\left(\frac{1}{m_e}\frac{\partial \ln\Psi}{\partial r_{1\mu}} - \frac{1}{m_h}\frac{\partial \ln\Psi}{\partial R_{a\mu}}\right)^2.$$

We calculate each derivative as:

$$\frac{\partial \ln \Psi}{\partial r_{1\mu}} = \frac{\partial \ln \psi_{\text{box}}}{\partial r_{1\mu}} + \frac{\partial \ln F}{\partial r_{1\mu}}, \quad \frac{\partial \ln \Psi}{\partial R_{a\mu}} = \frac{\partial \ln \psi_{\text{box}}}{\partial R_{a\mu}} + \frac{\partial \ln F}{\partial R_{a\mu}},$$

where:

$$\frac{\partial \ln \psi_{\text{box}}}{\partial x_i} = -k_x \tan(k_x x_i), \quad \frac{\partial \ln \psi_{\text{box}}}{\partial y_i} = -k_y \tan(k_y y_i), \quad \frac{\partial \ln \psi_{\text{box}}}{\partial z_i} = -k_z \tan(k_z z_i).$$

As for $\ln F$, it derives from terms like:

$$\frac{\partial \ln F}{\partial r_{1\mu}} = -\frac{Z}{2}\frac{\partial s_1}{\partial r_{1\mu}} + \frac{ZQ}{2} \tanh\left(\frac{ZQ}{2}(t_1 - t_2)\right)\frac{\partial t_1}{\partial r_{1\mu}} + Z\beta \frac{\partial}{\partial r_{1\mu}}\left(\frac{r_{12}}{1 + Z\alpha r_{12}}\right),$$

with:

$$\begin{aligned}
\frac{\partial s_1}{\partial r_{1\mu}} &= \frac{(r_{1\mu} - R_{a\mu})}{r_{1a}} + \frac{(r_{1\mu} - R_{b\mu})}{r_{1b}}, \\
\frac{\partial t_1}{\partial r_{1\mu}} &= \frac{(r_{1\mu} - R_{a\mu})}{r_{1a}} - \frac{(r_{1\mu} - R_{b\mu})}{r_{1b}}, \\
\frac{\partial}{\partial r_{1\mu}}\left(\frac{r_{12}}{1 + Z\alpha r_{12}}\right) &= \frac{(r_{1\mu} - r_{2\mu})}{r_{12}}\left(\frac{1}{1 + Z\alpha r_{12}} - \frac{Z\alpha r_{12}}{(1 + Z\alpha r_{12})^2}\right).
\end{aligned}$$

Combining the above expressions into a single compact equation yields:

$$\begin{aligned}
\frac{\partial \ln F}{\partial r_{1\mu}} = &-\frac{Z}{2}\left(\frac{r_{1\mu} - R_{a\mu}}{r_{1a}} + \frac{r_{1\mu} - R_{b\mu}}{r_{1b}}\right) \\
&+ \frac{ZQ}{2} \tanh\left[ZQ\frac{t_1 - t_2}{2}\right]\left(\frac{r_{1\mu} - R_{a\mu}}{r_{1a}} - \frac{r_{1\mu} - R_{b\mu}}{r_{1b}}\right) \\
&+ Z\beta \frac{1}{(1 + Z\alpha r_{12})^2}\frac{r_{1\mu} - r_{2\mu}}{r_{12}}.
\end{aligned}$$

Similarly, we calculate the derivatives of the distances with respect to $R_{a\mu}$:

$$\begin{aligned}
\frac{\partial s_1}{\partial R_{a\mu}} &= \frac{\partial r_{1a}}{\partial R_{a\mu}} + \frac{\partial r_{1b}}{\partial R_{a\mu}} = \frac{R_{a\mu} - r_{1\mu}}{r_{1a}} + 0 = \frac{R_{a\mu} - r_{1\mu}}{r_{1a}}, \\
\frac{\partial s_2}{\partial R_{a\mu}} &= \frac{\partial r_{2a}}{\partial R_{a\mu}} + \frac{\partial r_{2b}}{\partial R_{a\mu}} = \frac{R_{a\mu} - r_{2\mu}}{r_{2a}} + 0 = \frac{R_{a\mu} - r_{2\mu}}{r_{2a}}, \\
\frac{\partial t_1}{\partial R_{a\mu}} &= \frac{\partial r_{1a}}{\partial R_{a\mu}} - \frac{\partial r_{1b}}{\partial R_{a\mu}} = \frac{R_{a\mu} - r_{1\mu}}{r_{1a}} - 0 = \frac{R_{a\mu} - r_{1\mu}}{r_{1a}}, \\
\frac{\partial t_2}{\partial R_{a\mu}} &= \frac{\partial r_{2a}}{\partial R_{a\mu}} - \frac{\partial r_{2b}}{\partial R_{a\mu}} = \frac{R_{a\mu} - r_{2\mu}}{r_{2a}} - 0 = \frac{R_{a\mu} - r_{2\mu}}{r_{2a}}, \\
\frac{\partial r_{ab}}{\partial R_{a\mu}} &= \frac{R_{a\mu} - R_{b\mu}}{r_{ab}}.
\end{aligned}$$

Therefore,

$$\frac{\partial s_1 + s_2}{\partial R_{a\mu}} = \frac{R_{a\mu} - r_{1\mu}}{r_{1a}} + \frac{R_{a\mu} - r_{2\mu}}{r_{2a}},$$
$$\frac{\partial t_1 - t_2}{\partial R_{a\mu}} = \frac{R_{a\mu} - r_{1\mu}}{r_{1a}} - \frac{R_{a\mu} - r_{2\mu}}{r_{2a}}.$$

Then,

$$\begin{aligned}\frac{\partial \ln F}{\partial R_{a\mu}} &= -\frac{Z}{2}\frac{\partial s_1 + s_2}{\partial R_{a\mu}} + \frac{ZQ}{2}\tanh\left[ZQ\frac{t_1 - t_2}{2}\right]\frac{\partial t_1 - t_2}{\partial R_{a\mu}} \\ &+ Z\beta\frac{\partial}{\partial R_{a\mu}}\left(\frac{r_{ab}}{1 + Z\alpha r_{ab}}\right).\end{aligned}$$

Calculating the derivative of the last term:

$$\frac{\partial}{\partial R_{a\mu}}\left(\frac{r_{ab}}{1 + Z\alpha r_{ab}}\right) = \frac{1}{(1 + Z\alpha r_{ab})^2}\frac{R_{a\mu} - R_{b\mu}}{r_{ab}}.$$

Finally,

$$\begin{aligned}\frac{\partial \ln F}{\partial R_{a\mu}} &= -\frac{Z}{2}\left(\frac{R_{a\mu} - r_{1\mu}}{r_{1a}} + \frac{R_{a\mu} - r_{2\mu}}{r_{2a}}\right) \\ &+ \frac{ZQ}{2}\tanh\left[ZQ\frac{t_1 - t_2}{2}\right]\left(\frac{R_{a\mu} - r_{1\mu}}{r_{1a}} - \frac{R_{a\mu} - r_{2\mu}}{r_{2a}}\right) \\ &+ Z\beta\frac{1}{(1 + Z\alpha r_{ab})^2}\frac{R_{a\mu} - R_{b\mu}}{r_{ab}}.\end{aligned}$$

Thus, the full observable is:

$$\begin{aligned}O(\Psi(\mathbf{X})) = \sum_{\mu=1}^{3}\Bigg\{\frac{1}{m_e}\Bigg[&-k_\mu\tan(k_\mu r_{1\mu}) - \frac{Z}{2}\left(\frac{r_{1\mu} - R_{a\mu}}{r_{1a}} + \frac{r_{1\mu} - R_{b\mu}}{r_{1b}}\right) \\ &+ \frac{ZQ}{2}\tanh\left(\frac{ZQ}{2}(t_1 - t_2)\right)\left(\frac{r_{1\mu} - R_{a\mu}}{r_{1a}} - \frac{r_{1\mu} - R_{b\mu}}{r_{1b}}\right) \\ &+ Z\beta\frac{r_{1\mu} - r_{2\mu}}{r_{12}(1 + Z\alpha r_{12})^2}\Bigg] \\ &- \frac{1}{m_h}\Bigg[-k_\mu\tan(k_\mu R_{a\mu}) - \frac{Z}{2}\left(\frac{R_{a\mu} - r_{1\mu}}{r_{1a}} + \frac{R_{a\mu} - r_{2\mu}}{r_{2a}}\right) \\ &\quad + \frac{ZQ}{2}\tanh\left(\frac{ZQ}{2}(t_1 - t_2)\right)\left(\frac{R_{a\mu} - r_{1\mu}}{r_{1a}} - \frac{R_{a\mu} - r_{2\mu}}{r_{2a}}\right) \\ &\quad + Z\beta\frac{R_{a\mu} - R_{b\mu}}{r_{ab}(1 + Z\alpha r_{ab})^2}\Bigg]\Bigg\}^2\end{aligned}$$

[1] U. Roy, S. Ghosh and K. Bhattacharya, *Rev. Mex. Fis. E* 54 (2008) 160.

[2] Gil Paz, *Eur. J. Phys.* 22 (2001) 337.
